# Supplementary material for: Quantile Activation: Correcting a Failure Mode of ML Models
Source: arXiv:2405.11573 source file (2025-04-03)
Supplement: Supplementary file 1 [file fig_appendixA1.tex]

\begin{tikzpicture}
    % Axis
    \draw[thick,->] (0,0) -- (5.1,0) node[anchor=north west] {$\tau$};
    \draw[thick,->] (0,0) -- (0,5) node[anchor=south east] {};

    % Curved line (z_0 to z_1)
    \draw[domain=0:4,smooth,variable=\x,black,thick] plot ({\x},{0.25*\x^2 + 1});
    % \node at (-0.2,1) {$z_0$};
    \node at (4.4,5.4) {$F^{-1}(\tau)$};

    % Points on the line
    \coordinate (A) at (2.5,0.25*2.5^2 + 1);
    \coordinate (B) at (3.5,0.25*3.5^2 + 1);

    % Delta definitions
    \pgfmathsetmacro{\deltatau}{0.25}
    \pgfmathsetmacro{\zA}{0.25*2.5^2 + 1}
    \pgfmathsetmacro{\zB}{0.25*3.5^2 + 1}
    \pgfmathsetmacro{\deltaz}{\zB-\zA}

    % Drawing axes at points
    \draw[thin] (A) -- (2.5,0) node[below] {$\tau$};
    \draw[thin] (A) -- (0,0.25*2.5^2 + 1) node[left] {$z$};
    \draw[thin] (B) -- (3.5,0) node[below] {$\tau + \Delta \tau$};
    \draw[thin] (B) -- (0,0.25*3.5^2 + 1) node[left] {$z + \Delta z$};
    
    % Horizontal line and label
    \draw[dashed] (A) -- (3.5,0.25*2.5^2 + 1) node[midway,below] {$\Delta\tau$};
    \draw[dashed] (3.5,0.25*2.5^2 + 1) -- (B) node[midway,right] {$\Delta z$};

    % Diagonal line
    \draw[thick, red, dashed, shorten <=-1.5cm, shorten >=-1cm] (2.5,0.25*2.5^2 + 1) -- (3.5,0.25*2.5^2 + 1+1.25) node[midway,above,left] {$\frac{\partial F^{-1}(\tau)}{\partial \tau}$};
\end{tikzpicture}
